# Supplementary material for: Batch Reinforcement Learning with a Nonparametric Off-Policy Policy Gradient
Source: arXiv:2010.14771 source file (2021-06-07)
Supplement: Supplementary file 2 [file appendix.tex]

\section{Detail on the Theoretical Analysis}

\section{Detail on the Empirical Analysis}
\subsection{Gradient Analysis}

\subsection{Policy Improvement Analysis}
