# Supplementary material for: Batch Reinforcement Learning with a Nonparametric Off-Policy Policy Gradient
Source: arXiv:2010.14771 source file (2021-06-07)
Supplement: Supplementary file 7 [file appendix_backup.tex]

\onecolumn
%\begin{adjustwidth}{-75pt}{-60pt}

{\huge{Supplementary Material}}
%\section{Bias of Nadaraya-Watson Kernel Regression under Smoothness Assumptions}
%
%\begin{definition}{\emph{Lipschitz in $L_1$-normed space.}\\}
%	A function $f:\mathbb{R}^d\to \mathbb{R}$ is said to be Lipschitz continuous in the normed space with Lipschitz constant $L$ if and only if
%	\begin{equation}
%		|f(\svec_1)- f(\svec_2)| \leq |\svec_1 - \svec_2| L \quad \quad \forall \svec_1, \svec_2 \in \mathbb{R}^d. \nonumber
%	\end{equation}
%	where $|\cdot|$ is the norm in the $L_1$ space.
%	\label{lipschitz}
%\end{definition}
%
%\begin{definition}{\emph{Log-Lipschitz in $L_1$-normed space.}\\}
%	A positive defined function $f:\mathbb{R}^d\to \mathbb{R}$ is said to be log-Lipschitz continuous in the normed space with Lipschitz \\ constant $L$ if and only if
%	\begin{equation}
%		|\log f(\svec_1)- \log f(\svec_2)| \leq |\svec_1 - \svec_2| L \quad \quad \forall \svec_1, \svec_2 \in \mathbb{R}^d. \nonumber
%	\end{equation}
%	\label{loglipschitz}
%\end{definition}
%
%\begin{proposition}{\emph{Log-Lipschitz Distribution}\\}
%	There always exists a Lipschitz continuous function $g:\mathbb{R}^d\to\mathbb{R}$ with constant $L$ as defined in Definition~\ref{lipschitz} for any distribution with positive-defined Log-Lipschitz density $p$ defined over $\mathbb{R}^d$ with constant $L$ as defined in Definition~\ref{loglipschitz}, and
%	\begin{equation}
%		p(\svec) = \frac{\e{g(\svec)}}{\int_{-\infty}^{+\infty}\e{g(\svec)}\de \svec}. \nonumber
%	\end{equation}
%	\begin{proof}
%		When $g(\svec) = \log p(\svec)$
%		\begin{equation*}
%			p(\svec) = \frac{\e{\log p(\svec)}}{\int_{-\infty}^{+\infty}\e{\log p(\svec)}\de \svec} = \frac{p(\svec)}{\int_{-\infty}^{+\infty}p(\svec)\de \svec} =  p(\svec),
%		\end{equation*}
%		and $g(x)$ is Lipschitz with constant $L$ since $p$ is log-Lipschitz
%		\begin{equation}
%			|\log p(\svec_1) - \log p(\svec_2)| \leq |\svec_1 - \svec_2| L \implies |g(\svec_1) - g(\svec_2)| \leq |\svec_1 - \svec_2| L.\nonumber
%		\end{equation}
%	\end{proof}
%	\label{logdistribution}
%\end{proposition}
%
%\begin{proposition}
%	Given $\mathbf{h}, \mathbf{B} \in \mathbb{R}^d$, $L \in \mathbb{R}$
%	\begin{equation}
%		\int_{0}^{\Bvec}\prod_{i=1}^d \frac{\e{-\frac{\lvec_i^2}{2\hvec_i^2} - \lvec_i L_{\beta}}}{\sqrt{2\pi \hvec_i^2}}\de \lvec  = 2^{-d}\prod_{i=1}^d \e{\frac{L_{\beta}^2 h_i^2}{2}}\Bigg(\erf\bigg(\frac{ \Bvec_i + \hvec_i^2 L_{\beta}}{\hvec_i \sqrt{2}}\bigg) - \erf \bigg(\frac{\hvec_i L_{\beta}}{\sqrt{2}}\bigg) \Bigg), \nonumber
%	\end{equation}
%	where $\erf$ is the error-function.
%	\begin{proof}
%		\begin{align*}
%			\everymath={\displaystyle}
%			\int_{0}^{\Bvec}\prod_{i=1}^d \frac{\e{-\frac{\lvec_i^2}{2\hvec_i^2} - \lvec_i L_{\beta}}}{\sqrt{2\pi \hvec_i^2}}\de \lvec & = \prod_{i=1}^d \int_{0}^{\Bvec_i}  \frac{\e{-\frac{l_i^2}{2\hvec_i^2} - l L_{\beta}}}{\sqrt{2\pi \hvec_i^2}}\de l  \quad \quad \text{(Independent Factorization)} \\
%      		& = \prod_{i=1}^d \frac{1}{2} \e{\frac{L_{\beta}^2 \hvec_i^2}{2}} \Bigg[ 1 + \erf\bigg(\frac{ l + \hvec_i^2 L_{\beta}}{\hvec_i \sqrt{2}}\bigg) \Bigg]_{l=0}^{\Bvec_i} \\
%            & =  2^{-d}\prod_{i=1}^d \e{\frac{L_{\beta}^2 \hvec_i^2}{2}}\Bigg(\erf \bigg(\frac{ \Bvec_i + \hvec_i^2 L_{\beta}}{\hvec_i \sqrt{2}}\bigg) - \erf \bigg(\frac{\hvec_i L_{\beta}}{\sqrt{2}}\bigg) \Bigg).
%		\end{align*}
%	\end{proof}
%	\label{lipschitzgaussintegral}
%\end{proposition}
%
%\newpage
%
%\begin{proposition}
%	\begin{equation}
%		\int_{0}^{B}-\frac{\e{-\frac{l^2}{2\hvec_i^2} - l L_{\beta} }}{\sqrt{2\pi\hvec_i^2}}l L_{f} \de l = L_f \hvec_i \frac{\e{-\frac{B^2}{2\hvec_i^2} - B L_{\beta}} - 1}{2 \pi} + L_f L_{\beta}\hvec_i^2 \frac{\e{\frac{L_{\beta}^2 \hvec_i^2}{2}}}{2}\Bigg(\erf \bigg(\frac{ B + \hvec_i^2 L_{\beta}}{\hvec_i \sqrt{2}}\bigg) - \erf \bigg(\frac{\hvec_i L_{\beta}}{\sqrt{2}}\bigg) \Bigg) \nonumber
%	\end{equation}
%	\begin{proof}
%		\begin{eqnarray}
%			\int_{0}^{B}-\frac{\e{-\frac{l^2}{2\hvec_i^2}- l L_{\beta} }}{\sqrt{2\pi\hvec_i^2}}l L_f \de l & = & \frac{L_f\hvec_i}{\sqrt{2\pi}}  \int_{0}^{B}-\frac{l}{\hvec_i^2} \e{-\frac{l^2}{2\hvec_i^2}- l L_{\beta} }\de l \nonumber \\
%			& = &  \frac{L_f \hvec_i}{\sqrt{2\pi}}  \bigg(\underbrace{\int_{0}^{B}\bigg(-\frac{l}{\hvec_i^2}-L_{\beta}\bigg)  \e{-\frac{l^2}{2\hvec_i^2}- l L_{\beta} }\de l}_{\text{Integral 1}} + L_{\beta}\sqrt{2\pi\hvec_i^2}\underbrace{\int_{0}^B \frac{\e{-\frac{l^2}{2\hvec_i^2}- l L_{\beta} }}{\sqrt{2\pi\hvec_i^2}}\de l}_{\text{Integral 2}}\bigg)\nonumber \\ \label{parprop3}
%		\end{eqnarray}
%		The solution of Integral~1 is
%		\begin{equation*}
%			\int_{0}^{B}\bigg(-\frac{l}{\hvec_i^2}-L_{\beta}\bigg) \e{-\frac{l^2}{2\hvec_i^2}- l L_{\beta} }\de l = \Bigg[\e{-\frac{l^2}{2\hvec_i^2}- l L_{\beta} }\Bigg]_{l=0}^B = \e{-\frac{B^2}{2\hvec_i^2}- B L_{\beta} }- 1, \nonumber
%		\end{equation*}
%		and based on Proposition~\ref{lipschitzgaussintegral} the second integral is
%		\begin{equation}
%			\int_{0}^B\frac{\e{-\frac{l^2}{2\hvec_i^2}- l L_{\beta} }}{\sqrt{2\pi\hvec_i^2}}\de l = \frac{ \e{\frac{L_{\beta}^2 \hvec_i^2}{2}}}{2}\Bigg(\erf\bigg(\frac{ B + \hvec_i^2 L_{\beta}}{\hvec_i \sqrt{2}}\bigg) - \erf\bigg(\frac{\hvec_i L_{\beta}}{\sqrt{2}}\bigg) \Bigg). \nonumber
%		\end{equation}
%		Plugging back in Equation~\eqref{parprop3}
%		\begin{eqnarray}
%			\int_{0}^{B}-\frac{\e{-\frac{l^2}{2\hvec_i^2}- l L_{\beta} }}{\sqrt{2\pi\hvec_i^2}}l L_f \de l\nonumber &=&  \frac{L_f\hvec_i}{\sqrt{2\pi}}  \Bigg(\e{-\frac{B^2}{2\hvec_i^2}- B L_{\beta} }-1 + L_{\beta}\sqrt{2\pi\hvec_i^2} \frac{\e{\frac{L_{\beta}^2 \hvec_i^2}{2}}}{2}\Bigg(\erf\bigg(\frac{ B + \hvec_i^2 L_{\beta}}{\hvec_i \sqrt{2}}\bigg) - \erf\bigg(\frac{\hvec_i L_{\beta}}{\sqrt{2}}\bigg) \Bigg) \Bigg) \nonumber\\
%			& = & L_f\hvec_i \frac{\e{-\frac{B^2}{2\hvec_i^2}- B L_{\beta} }-1}{\sqrt{2 \pi} } + L_f L_{\beta}\hvec_i^2 \frac{\e{\frac{L_{\beta}^2 \hvec_i^2}{2}}}{2}\Bigg(\erf\bigg(\frac{ B + \hvec_i^2 L_{\beta}}{\hvec_i \sqrt{2}}\bigg) - \erf\bigg(\frac{\hvec_i L_{\beta}}{\sqrt{2}}\bigg) \Bigg). \nonumber
%		\end{eqnarray}
%	\end{proof}
%	\label{preposition3}
%\end{proposition}
%
%\newpage
%
%\begin{proposition}
%	Given $\Avec, \Bvec \in \mathbb{R}^d$,
%	\begin{equation}
%		\int_\Avec^\Bvec \bigg(\prod_{i=1}^d f(\svec_i)\bigg)\bigg(\sum_{k=1}^dg(\svec_k)\bigg) \de \svec = \sum_{k=1}^d \bigg(\prod_{i\neq k}^d\int_{\Avec_i}^{\Bvec_i}f(x)\de x \bigg)\int_{\Avec_k}^{\Bvec_k}f(x)g(x)\de x. \nonumber
%	\end{equation}
%	\begin{proof}
%		\begin{eqnarray}
%			\int_\Avec^\Bvec \bigg(\prod_{i=1}^d f(\svec_i)\bigg)\bigg(\sum_{k=1}^dg(\svec_k)\bigg) \de \svec &=&\sum_{k=1}^d \int_\Avec^\Bvec \bigg(\prod_{i=1}^d f(\svec_i)\bigg)g(\svec_k) \de \svec \nonumber \\
%			&=&\sum_{k=1}^d \int_\Avec^\Bvec  f(\svec_1)f(\svec_2)\dots f(\svec_d)g(\svec_k) \de \svec \nonumber \\
%			&=&\sum_{k=1}^d \int_{\Avec_1}^{\Bvec_1} f(x)\de x \int_{\Avec_2}^{\Bvec_2} f(x)\de x\dots\nonumber \\
%			& & \quad \quad \int_{\Avec_n}^{\Bvec_n} f(x)\de x   \int_{\Avec_k}^{\Bvec_k} f(x)g(x)\de x \nonumber \\
%			&=& \sum_{k=1}^d \bigg(\prod_{i\neq k}^d\int_{\Avec_i}^{\Bvec_i}f(x)\de x \bigg)\int_{\Avec_k}^{\Bvec_k}f(x)g(x)\de x \nonumber
%		\end{eqnarray}
%	\end{proof}
%	\label{prodsumint}
%\end{proposition}
%
%\begin{definition}{A multivariate Gaussian Kernel with bandwidth $\hvec \in \mathbb{R}$ is defined as}
%	\begin{equation}
%		K(\svec, \zvec) = \prod_{i=1}^d\frac{\e{-\frac{(\svec_i-\zvec_i)^2}{2\hvec_i^2}}}{\sqrt{2\pi\hvec_i^2}}. \nonumber
%	\end{equation}
%	\label{kerdef}
%\end{definition}
%
%\begin{definition}{Nadaraya-Watson Kernel Regression.}
%	We define the Nadaraya-Watson Kernel Regression with Gaussian Kernels (as defined in Definition~\ref{kerdef}) of a data-set $\{\svec_i, y_i\}_{i=1}^n$ as
%	\begin{equation}
%		\approxx{f}_n(\svec) = \frac{\sum_{i=1}^nK(\svec, \svec_i)y_i}{\sum_{j=1}^nK(\svec, \svec_j)}. \nonumber
%	\end{equation}
%\end{definition}
%
%
%\textbf{Theorem~\ref{theorem:biasnadaraya}} \emph{Bias of Nadaraya-Watson Kernel Regression under Smooth Assumptions.}
%\begin{proof}
%	Substituting the Definition~\ref{kerdef} on the left-side
%	\begin{eqnarray}
%		\bigg|\EV\Big[\lim_{n\to \infty}\approxx{f}_n(\svec) \Big] - f(\svec)\bigg| & = & \bigg|\EV\bigg[\lim_{n\to \infty}\frac{\sum_{i=1}^nK(\svec, \svec_i)y_i}{\sum_{j=1}^nK(\svec, \svec_j)} \bigg] - f(\svec)\bigg| \nonumber \\
%		& = & \bigg|\EV\bigg[\lim_{n\to \infty}\frac{n^{-1}\sum_{i=1}^nK(\svec, \svec_i)y_i}{n^{-1}\sum_{j=1}^nK(\svec, \svec_j)} \bigg] - f(\svec)\bigg| \nonumber \\
%		& = & \bigg|\EV\bigg[\frac{\int_{-\infty}^{\infty}K(\svec, \zvec)\big(f(\zvec) + \epsilon(\zvec)\big)\beta(\zvec)\de \zvec}{\int_{-\infty}^{+\infty}K(\svec, \zvec)\beta(\zvec)\de \zvec} \bigg] - f(\svec)\bigg| \nonumber \\
%		& = & \bigg|\frac{\int_{-\infty}^{+\infty}\int_{-\infty}^{\infty}K(\svec, \zvec)\big(f(\zvec) + \int_{-\infty}^{+\infty}\epsilon_\zvec\de \epsilon_\zvec  \big)\beta(\zvec)\de\zvec}{\int_{-\infty}^{+\infty}K(\svec, \zvec)\beta(\zvec)\de \zvec}- f(\svec)\bigg| \label{equation:noiseclear}\\
%		& = & \bigg|\frac{\int_{-\infty}^{\infty}K(\svec, \zvec)f(\zvec) \beta(\zvec)\de \zvec}{\int_{-\infty}^{+\infty}K(\svec, \zvec)\beta(\zvec)\de \zvec} - f(\svec)\bigg| \nonumber \\
%		& = & \bigg|\frac{\int_{-\infty}^{\infty}K(\svec, \zvec)\big(f(\zvec)- f(\svec) \big)\beta(\zvec)\de \zvec}{\int_{-\infty}^{+\infty}K(\svec, \zvec)\beta(\zvec)\de \zvec}\bigg| \label{equation:kerregwonoise} \\
%		& = & \frac{\big|\int_{-\infty}^{\infty}K(\svec, \zvec)\big(f(\zvec)- f(\svec) \big)\beta(\zvec)\de \zvec\big|}{\big|\int_{-\infty}^{+\infty}K(\svec, \zvec)\beta(\zvec)\de \zvec\big|}. \nonumber
%	\end{eqnarray}
%	We want to obtain an upper-bound of the bias. Therefore we want to find an upper-bound of the numerator and a lower-bound of the denominator. Note that the magnitude of the noise does not influence the Bias \cite{wasserman_all_2006}.
%	\paragraph{Lower-bound of the Denominator:}
%	The denominator is always positive, so the absolute value operator can be removed,
%	\begin{eqnarray}
%		\int_{-\infty}^{+\infty}K(\svec, \zvec)\beta(\zvec)\de \zvec & = & \int_{-\infty}^{+\infty}\prod_{i=1}^d\frac{\e{-\frac{(\svec_i-\zvec_i)^2}{2\hvec_i^2}}}{\sqrt{2\pi\hvec_i^2}}\beta(\zvec)\de \zvec \nonumber \\
%		& = & \frac{1}{\int_{-\infty}^{\infty}\e{g(\zvec)}\de \zvec}\int_{-\infty}^{+\infty}\prod_{i=1}^d\frac{\e{-\frac{(\svec_i-\zvec_i)^2}{2\hvec_i^2}}}{\sqrt{2\pi\hvec_i^2}}\e{g(\zvec)}\de \zvec \nonumber \\
%		& = & \frac{\e{g(\svec)}}{\int_{-\infty}^{\infty}\e{g(\zvec)}\de \zvec}\int_{-\infty}^{+\infty}\bigg(\prod_{i=1}^d\frac{\e{-\frac{(\svec_i-\zvec_i)^2}{2\hvec_i^2}}}{\sqrt{2\pi\hvec_i^2}}\bigg)\e{g(\zvec)-g(\svec)}\de \zvec\nonumber \\
%		& = & \frac{\e{g(\svec)}}{\int_{-\infty}^{\infty}\e{g(\zvec)}\de \zvec}\int_{-\infty}^{+\infty}\bigg(\prod_{i=1}^d\frac{\e{-\frac{\lvec_i^2}{2\hvec_i^2}}}{\sqrt{2\pi\hvec_i^2}}\bigg)\e{g(\svec+\lvec)-g(\svec)}\de \lvec  \qquad \text{(let $l = x - z$)} \nonumber \\
%		& \geq & \frac{\e{g(\svec)}}{\int_{-\infty}^{\infty}\e{g(\zvec)}\de \zvec}\int_{-\infty}^{+\infty}\bigg(\prod_{i=1}^d\frac{\e{-\frac{\lvec^2}{2\hvec_i^2}}}{\sqrt{2\pi\hvec_i^2}}\bigg)\e{-|\lvec|L_{\beta}}\de \lvec  \nonumber \\
%		& = & \frac{\e{g(\svec)}}{\int_{-\infty}^{\infty}\e{g(\zvec)}\de \zvec}\int_{-\infty}^{+\infty}\bigg(\prod_{i=1}^d\frac{\e{-\frac{\lvec_i^2}{2\hvec_i^2}}}{\sqrt{2\pi\hvec_i^2}}\bigg)\bigg(\prod_{j=1}^d \e{-|\lvec_j|L_{\beta}}\bigg)\de \lvec  \qquad \text{(Lipschitz Inequality)} \nonumber  \\
%		& = & 2^d\frac{\e{g(\svec)}}{\int_{0}^{\infty}\e{g(\zvec)}\de \zvec}\int_{0}^{+\infty}\bigg(\prod_{i=1}^d\frac{\e{-\frac{\lvec_i^2}{2\hvec_i^2}}}{\sqrt{2\pi\hvec_i^2}}\bigg)\bigg(\prod_{j=1}^d \e{-\lvec_j L_{\beta}}\bigg)\de \lvec \qquad \text{(Symmetric Integral)} \nonumber \\
%		& = & 2^d\frac{\e{g(\svec)}}{\int_{0}^{\infty}\e{g(\zvec)}\de \zvec}\int_{0}^{+\infty}\prod_{i=1}^d\frac{\e{-\frac{\lvec_i^2}{2\hvec_i^2}-\lvec_i L_{\beta}}}{\sqrt{2\pi\hvec_i^2}}\de \lvec.  \nonumber
%	\end{eqnarray}
%	Now considering Proposition~\ref{lipschitzgaussintegral}, we obtain
%	\begin{equation}
%		\int_{-\infty}^{+\infty}K(\svec, \zvec)\beta(\zvec)\de \zvec \leq \frac{\e{g(\svec)}}{\int_{-\infty}^{\infty}\e{g(\zvec)}\de \zvec}\prod_{i=1}^d  \e{\frac{L_{\beta}^2 h_i^2}{2}}\Bigg(1 - \erf\bigg(\frac{\hvec_i L_{\beta}}{\sqrt{2}}\bigg) \Bigg).
%		\label{denominator}
%	\end{equation}
%	\newpage
%	\paragraph{Upper-bound of the Numerator:}
%	\begin{eqnarray}
%		&   & \bigg|\int_{-\infty}^{\infty}K(\svec, \zvec)\big(f(\zvec)- f(\svec) \big)\beta(\zvec)\de \zvec\bigg| \nonumber \\
%		& = & \bigg|\int_{-\infty}^{\infty}K(\svec, \svec + \lvec)\big(f(\svec+\lvec)- f(\svec) \big)\beta(\svec+\lvec)\de \lvec\bigg| \nonumber \\
%		& \leq & \int_{-\infty}^{\infty}K(\svec, \svec + \lvec)\big|f(\svec+\lvec)- f(\svec) \big|\beta(\svec+\lvec)\de \lvec \nonumber \\
%		& = & \frac{1}{\int_{-\infty}^{\infty}\e{g(\zvec)}\de \zvec}\int_{-\infty}^{\infty}K(\svec, \svec + \lvec)\big|f(\svec+\lvec)- f(\svec) \big|\e{g(\svec+\lvec)}\de \lvec \qquad \text{(Jensen's Inequality)} \nonumber \\
%		& \leq & \frac{1}{\int_{-\infty}^{\infty}\e{g(\zvec)}\de \zvec}\int_{-\infty}^{\infty}K(\svec, \svec + \lvec)\big|\lvec \big| L_{f} \e{g(\svec+\lvec)}\de \lvec \qquad \text{(Lipschitz Inequality)}  \nonumber \\
%		& = & \frac{1}{\int_{-\infty}^{\infty}\e{g(\zvec)}\de \zvec}\int_{-\infty}^{\infty}K(\svec, \svec + \lvec)\sum_{i=1}^{n}\big|\lvec_i \big| L_{f} \e{g(\svec+\lvec)}\de \lvec \nonumber \\
%		& = & \frac{\e{g(\svec)}}{\int_{-\infty}^{\infty}\e{g(\zvec)}\de \zvec}\int_{-\infty}^{\infty}K(\svec, \svec + \lvec)\sum_{i=1}^{n}\big|\lvec_i \big| L_{f} \e{g(\svec+\lvec)-g(\svec)}\de \lvec \nonumber \\
%		& \leq & \frac{\e{g(\svec)}}{\int_{-\infty}^{\infty}\e{g(\zvec)}\de \zvec}\int_{-\infty}^{\infty}K(\svec, \svec + \lvec)\sum_{i=1}^{n}\big|\lvec_i \big| L_{f} \prod_{i=1}^d \e{|\lvec_i|L_{\beta}}\de \lvec \nonumber \\
%		& = & \frac{\e{g(\svec)}}{\int_{-\infty}^{\infty}\e{g(\zvec)}\de \zvec}\int_{-\infty}^{\infty}\Bigg(\prod_{i=1}^d\frac{\e{-\frac{\lvec^2}{2\hvec_i^2}}}{\sqrt{2\pi\hvec_i^2}}\Bigg)\sum_{i=1}^{n}\big|\lvec_i \big| L_{f} \prod_{i=1}^d \e{|\lvec_i|L_{\beta}}\de \lvec \nonumber \\
%		& = & 2^d \frac{\e{g(\svec)}}{\int_{-\infty}^{\infty}\e{g(\zvec)}\de \zvec}\int_{0}^{\infty}\Bigg(\prod_{i=1}^d\frac{\e{-\frac{\lvec^2}{2\hvec_i^2}+ \lvec_i L_{\beta} }}{\sqrt{2\pi\hvec_i^2}}\Bigg)\sum_{i=1}^{n}\lvec_i L_{f} \de \lvec. \nonumber
%	\end{eqnarray}
%	Using Proposition~\ref{prodsumint},
%	\begin{eqnarray}
%		& & 2^d \frac{\e{g(\svec)}}{\int_{-\infty}^{\infty}\e{g(\zvec)}\de \zvec}\int_{0}^{+\infty}\Bigg(\prod_{i=1}^d\frac{\e{-\frac{\lvec^2}{2\hvec_i^2}+  \lvec_i L_{\beta} }}{\sqrt{2\pi\hvec_i^2}}\Bigg)\sum_{i=1}^{n}\lvec_i  L_{f} \de \lvec \nonumber \\
%		& = &  2^d \frac{\e{g(\svec)}}{\int_{-\infty}^{\infty}\e{g(\zvec)}\de \zvec}\sum_{k=1}^d \bigg(\prod_{i\neq k}^d\int_{0}^{+\infty}\frac{\e{-\frac{l^2}{2\hvec_i^2}+ l L_{\beta} }}{\sqrt{2\pi\hvec_i^2}}\de l \bigg)\int_{0}^{+\infty}\frac{\e{-\frac{l^2}{2\hvec_k^2}+ l L_{\beta} }}{\sqrt{2\pi\hvec_k^2}}l L_{f} \de l \nonumber \\
%		& = & 2^d \frac{\e{g(\svec)}}{\int_{-\infty}^{\infty}\e{g(\zvec)}\de \zvec} \sum_{k=1}^d \bigg(\prod_{i\neq k}^d\int_{0}^{-\infty}-\frac{\e{-\frac{l^2}{2\hvec_i^2}- l L_{\beta} }}{\sqrt{2\pi\hvec_i^2}}\de l \bigg)\int_{0}^{-\infty}\frac{\e{-\frac{l^2}{2\hvec_k^2}- l L_{\beta} }}{\sqrt{2\pi\hvec_k^2}}l L_{f} \de l. \nonumber
%	\end{eqnarray}
%	Using Proposition~\ref{lipschitzgaussintegral},
%	\begin{eqnarray}
%		& = & 2^d \frac{\e{g(\svec)}}{\int_{-\infty}^{\infty}\e{g(\zvec)}\de \zvec} \sum_{k=1}^d \Bigg(2^{-d}\prod_{i\neq k}^d \e{\frac{L_{\beta}^2 \hvec_i^2}{2}}\Bigg(1 +  \erf\bigg(\frac{\hvec_i L_{\beta}}{\sqrt{2}}\bigg) \Bigg)\Bigg)\int_{0}^{-\infty}\frac{\e{-\frac{l^2}{2\hvec_k^2}- l L_{\beta} }}{\sqrt{2\pi\hvec_k^2}}l L_{f} \de l \nonumber \\
%		& = & \frac{\e{g(\svec)}}{\int_{-\infty}^{\infty}\e{g(\zvec)}\de \zvec} \sum_{k=1}^d \Bigg(\prod_{i\neq k}^d \e{\frac{L_{\beta}^2 \hvec_i^2}{2}}\Bigg(1 +  \erf\bigg(\frac{\hvec_i L_{\beta}}{\sqrt{2}}\bigg) \Bigg)\Bigg)\int_{0}^{-\infty}\frac{\e{-\frac{l^2}{2\hvec_k^2}- l L_{\beta} }}{\sqrt{2\pi\hvec_k^2}}l L_{f} \de l. \nonumber
%	\end{eqnarray}
%	Using Proposition~\ref{preposition3} to solve the last integral
%	\begin{eqnarray}
%		&=&\frac{\e{g(\svec)}}{\int_{-\infty}^{\infty}\e{g(\zvec)}\de \zvec} \sum_{k=1}^d \Bigg(\prod_{i\neq k}^d \e{\frac{L_{\beta}^2 \hvec_i^2}{2}}\Bigg(1 +  \erf \bigg(\frac{\hvec_i L_{\beta}}{\sqrt{2}}\bigg) \Bigg)\Bigg) \nonumber \\
%		& & \quad \quad \quad \times L_{f}\hvec_k \Bigg( \frac{1}{\sqrt{2 \pi} } + L_{\beta}\hvec_k \frac{\e{\frac{L_{\beta}^2 \hvec_k^2}{2}}}{2}\Bigg(1 + \erf \bigg(\frac{\hvec_k L_{\beta}}{\sqrt{2}}\bigg) \Bigg)\Bigg). \nonumber \\
%		\label{numerator}
%	\end{eqnarray}
%	\paragraph{Conclusion.}
%	Unifying equations \eqref{numerator} and \eqref{denominator} we finally obtain
%	\begin{eqnarray}
%		& & \bigg|\EV\Big[\lim_{n\to \infty}\approxx{f}_n(\svec) \Big] - f(\svec)\bigg| \leq \nonumber \\  & & \frac{L_f \sum\limits_{k=1}^d \hvec_k \Bigg(\prod\limits_{i\neq k}^d \e{\frac{L_{\beta}^2 \hvec_i^2}{2}}\Bigg(1 +  \erf\bigg(\frac{\hvec_i L_{\beta}}{\sqrt{2}}\bigg) \Bigg)\Bigg)  \Bigg( \frac{1}{\sqrt{2 \pi} } + L_{\beta}\hvec_k \frac{\e{\frac{L_{\beta}^2 \hvec_k^2}{2}}}{2}\Bigg(1 + \erf\bigg(\frac{\hvec_k L_{\beta}}{\sqrt{2}}\bigg) \Bigg)\Bigg)}{\prod\limits_{i=1}^d  \e{\frac{L_{\beta}^2 h_i^2}{2}}\Bigg(1 - \erf\bigg(\frac{\hvec_i L_{\beta}}{\sqrt{2}}\bigg) \Bigg)}. \nonumber
%	\end{eqnarray}
%\end{proof}
%
%
%\newpage 

\section{The Nonparametric Bellman Equation}
This section contains the proofs of Theorem~\ref{theorem:fixedpoint} and Theorem~\ref{theorem:ultimate}. \\
\begin{proposition}
	In the limit of infinite samples the NPBE defined in Definition~\ref{definition:npbe} with a data-set $\lim_{n\to \infty}D_n$ collected under distribution $\beta$ on the state-action space and MDP $\mathcal{M}$ converges to
	\begin{eqnarray}
		\approxx{V}_{\pi}(\svec)  & = &  \int_{\Sset \times \Aset} \varepsilon_{\pi}(\svec,\zvec, \bvec) \bigg( R_{\zvec, \bvec} + \gamma \int_{\Sset}\approxx{V}_{\pi}(\svec')\phi(\svec', \zvec_{\zvec, \bvec}')\de \svec'  \bigg) \beta(\zvec, \bvec) \de \zvec \de \bvec, \nonumber \\
		& & \text{with} \quad R_{\zvec, \bvec} \sim R(\zvec, \bvec) \quad \forall(\zvec, \bvec) \in \Sset \times \Aset, \nonumber \\
		& & \text{with} \quad \zvec_{\zvec, \bvec}' \sim P(\cdot |\zvec, \bvec) \quad \forall(\zvec, \bvec) \in \Sset \times \Aset. \label{equation:infnpbe}
	\end{eqnarray}
	and
	\begin{equation}
		\begin{cases}
			\varepsilon_{\pi}(\svec, \zvec, \bvec) \defeq \bigintsss_{\Aset} \displaystyle \frac{\psi(\svec, \zvec)\varphi(\avec, \bvec)}{\int_{\Sset, \Aset}\psi(\svec, \zvec)\varphi(\avec, \bvec)\beta(\zvec, \bvec) \de \zvec \de \bvec} \pi(\avec | \svec) \de \avec & \text{if $\pi$ is stochastic}, \\
			\\
			\varepsilon^{\pi}_i(\svec)  \defeq \displaystyle \frac{\psi(\svec, \zvec)\varphi(\pi(\svec),\bvec)}{\int_{\Sset, \Aset} \psi(\svec, \zvec)\varphi(\pi(\svec), \bvec)\beta(\zvec, \bvec) \de \zvec \de \bvec}                                           & \text{otherwise.}
		\end{cases}\nonumber
	\end{equation}
	\begin{proof}
		\begin{eqnarray}
			\approxx{V}_{\pi}(\svec) & = & \lim_{n \to \infty} \int_{\Aset}\frac{\sum_{i=1}^n\psi_i(\svec)\varphi_i(\avec)\bigg(r_i + \gamma \int_{\Sset}\phi_i(\svec')\approxx{V}_{\pi}(\svec')\de \svec\bigg)}{\sum_{i=1}^n\psi_j(\svec)\varphi_j(\avec)} \pi(\avec | \svec) \de \avec \nonumber \\
			& = & \int_{\Aset}\frac{\lim_{n \to \infty}\frac{1}{n}\sum_{i=1}^n\psi_i(\svec)\varphi_i(\avec)\bigg(r_i + \gamma \int_{\Sset}\phi_i(\svec')\approxx{V}_{\pi}(\svec')\de \svec\bigg)}{\lim_{n \to \infty} \frac{1}{n}\sum_{i=1}^n\psi_j(\svec)\varphi_j(\avec)} \pi(\avec | \svec) \de \avec \nonumber \\
			& = & \int_{\Aset}\frac{\int_{\Sset \times \Aset}\psi(\svec, \zvec)\varphi(\avec, \bvec)\bigg( R(\zvec, \bvec) + \gamma \int_{\Sset}\phi(\svec', \zvec')p(\zvec'|\bvec, \zvec)\approxx{V}_{\pi}(\svec')\de \svec  \bigg) \beta(\zvec, \bvec) \de \zvec \de \bvec}{\int_{\Sset \times \Aset}\psi(\svec, \zvec)\varphi(\avec, \bvec)\beta(\zvec, \bvec) \de \zvec \de \bvec} \pi(\avec | \svec) \de \avec. \nonumber
		\end{eqnarray}
		Analogously we can derive the deterministic policy case.
	\end{proof}
\end{proposition}

\begin{proposition}
	Both for finite samples and infinite samples, when $R$ is bounded by $-R_\text{max}$ and $R_\text{max}$ (where $R_\text{max}$ is non-negative defined), then the solution of the NPBE if exists it is bounded between $\frac{-2R_\text{max}}{1-\gamma}$ and $\frac{2R_\text{max}}{1-\gamma}$.
	\begin{proof}
		Starting with the finite samples case. Suppose by absurd proposition that if the NPBE admits a solution $\approxx{V}_{\pi}$ then $\sup_{\svec}|\approxx{V}_{\pi}(\svec)| =  \frac{R_\text{max}}{1-\gamma} + \epsilon $ with $\epsilon > 0$ strictly positive (and eventually $+\infty$).
		It immediately follows that $\sup_{\svec_1, \svec_2}|\approxx{V}_{\pi}(\svec_1) - \approxx{V}_{\pi}(\svec_2) | =  \frac{2R_\text{max}}{1-\gamma} + 2 \epsilon $.
		Expanding this term
		\begin{eqnarray}
			\sup_{\svec_1, \svec_2}|\approxx{V}_{\pi}(\svec_1) - \approxx{V}_{\pi}(\svec_2) | & = &  \sup_{\svec_1, \svec_2} \bigg|\bigg(\bm{\varepsilon}_{\pi}^{T}(\svec_1)-\bm{\varepsilon}_{\pi}^{T}(\svec_2)\bigg)\bigg(\rvec + \gamma \int_{\Sset} \phivec(\svec')\approxx{V}_{\pi}(\svec')   \de \svec'\bigg)\bigg| \nonumber \\
			& \leq &  \sup_{\svec_1, \svec_2} \bigg|\bm{\varepsilon}_{\pi}^{T}(\svec_1)-\bm{\varepsilon}_{\pi}^{T}(\svec_2)\bigg|\bigg|\rvec + \gamma \int_{\Sset} \phivec(\svec')\approxx{V}_{\pi}(\svec')   \de \svec'\bigg| \nonumber \\
			& \leq &  \sup_{\svec_1, \svec_2} \bigg(\big|\bm{\varepsilon}_{\pi}^{T}(\svec_1)\big|+\big|\bm{\varepsilon}_{\pi}^{T}(\svec_2)\big|\bigg)\bigg|\rvec + \gamma \int_{\Sset} \phivec(\svec')\approxx{V}_{\pi}(\svec')   \de \svec'\bigg|. \nonumber
		\end{eqnarray}
		Notice that $\bm{\varepsilon}_{\pi}^T(\svec)$ is a stochastic vector (non-negative definite and sums up to 0),
		\begin{eqnarray}
			& & \sup_{\svec_1, \svec_2} \bigg(\big|\bm{\varepsilon}_{\pi}^{T}(\svec_1)\big|+\big|\bm{\varepsilon}_{\pi}^{T}(\svec_2)\big|\bigg)\bigg|\rvec + \gamma \int_{\Sset} \phivec(\svec')\approxx{V}_{\pi}(\svec')   \de \svec'\bigg| \nonumber \\
			& \leq & 2 R_\text{max} +\gamma \sup_{\svec_1, \svec_2} \bigg(\big|\bm{\varepsilon}_{\pi}^{T}(\svec_1)\big|+\big|\bm{\varepsilon}_{\pi}^{T}(\svec_2)\big|\bigg)\bigg|  \int_{\Sset} \phivec(\svec')\approxx{V}_{\pi}(\svec')   \de \svec'\bigg| \nonumber \\
			& \leq & 2 R_\text{max} +\gamma \bigg(\frac{R_\text{max}}{1-\gamma} + \epsilon\bigg) \sup_{\svec_1, \svec_2} \bigg(\big|\bm{\varepsilon}_{\pi}^{T}(\svec_1)\big|+\big|\bm{\varepsilon}_{\pi}^{T}(\svec_2)\big|\bigg) \int_{\Sset} \phivec(\svec')  \de \svec' \nonumber \\
			& = & 2 R_\text{max} +\gamma \bigg(\frac{R_\text{max}}{1-\gamma} + \epsilon\bigg)  \sup_{\svec_1, \svec_2} \bigg(\big|\bm{\varepsilon}_{\pi}^{T}(\svec_1)\big|+\big|\bm{\varepsilon}_{\pi}^{T}(\svec_2)\big|\bigg) \mathbf{1} \nonumber \\
			& \leq & 2 R_\text{max} +\gamma \bigg(\frac{2 R_\text{max}}{1-\gamma} + 2 \epsilon\bigg),   \nonumber
		\end{eqnarray}
		which implies that
		\begin{eqnarray}
			\sup_{\svec_1, \svec_2}|\approxx{V}_{\pi}(\svec_1) - \approxx{V}_{\pi}(\svec_2) | & \leq &   2 R_\text{max} +\gamma \bigg(\frac{2 R_\text{max}}{1-\gamma} + 2 \epsilon\bigg)   \nonumber \\
			\implies 2 \frac{R_\text{max}}{1-\gamma} + 2 \epsilon & \leq &   2 R_\text{max} +\gamma \bigg(\frac{2 R_\text{max}}{1-\gamma} + 2 \epsilon\bigg)   \nonumber \\
			\implies 0 \leq \epsilon\big(\gamma(1-\gamma) - 1\big).
		\end{eqnarray}
		Since $\gamma(1- \gamma) - 1$ is always negative (we defined $0 \leq \gamma < 1$), then there are no positive values for $\epsilon$ which satisfy the inequality, which is in clear contradiction with the absurd premise.
		For the infinite samples case we can do similar reasoning noting that $\phi, \beta, P$ are probability measures.
	\end{proof}
\end{proposition}

\begin{proposition}
	\label{proposition:uniqueness}
	If $R$ is bounded by $R_{\text{max}}$ and if $f^*:\Sset \to \mathbb{R}$ satisfies the NPBE, then there is no other function $f:\Sset \to \mathbb{R}$ for which $\exists \zvec \in \Sset$ and $|f^*(\zvec) - f(\zvec)| > 0$.
	\begin{proof}
		Suppose, by absurd assumption, that a function $g:\Sset \to \mathbb{R}$ exists such that $f(\svec) + g(\svec)$ satisfies Equation~\eqref{equation:infnpbe} for every $\svec \in \Sset$ and a constant $G \in \mathbb{R}^+$ exists for which $|g(\zvec)| > G$.
		Note that the existence of $f:\Sset\to\mathbb{R}$ as a solution for the NPBE implies the existence of
		\begin{equation}
			\int_{\Sset}\bm{\varepsilon}_{\pi}^T(\svec)\phivec(\svec')f^*(\svec ' )\de   \svec ' \in \mathbb{R}, \label{equation:existenceint1}
		\end{equation}
		and similarly, the existence of $f(\svec) \in \mathbb{R}$ with $f(\svec) = f^*(\svec) + g(\svec)$ as a solution of the NPBE implies that
		\begin{equation}
			\int_{\Sset}\bm{\varepsilon}_{\pi}^T(\svec)\phivec(\svec')f^*(\svec ' ) + g(\svec')\de   \svec ' \in \mathbb{R}. \label{equation:existenceint2}
		\end{equation}
		Note that the existence of the integral in Equations~\eqref{equation:existenceint1} and \eqref{equation:existenceint2} implies
		\begin{equation}
			\int_{\Sset}\bm{\varepsilon}_{\pi}^T(\svec)\phivec(\svec') g(\svec')\de   \svec ' \in \mathbb{R}. \label{equation:existenceint3}
		\end{equation}
		Note that
		\begin{eqnarray}
			|f^*(\svec) - f(\svec)| & = & \bigg| f^*(\svec) - \bm{\varepsilon}_{\pi}^T(\svec) \bigg(\rvec + \gamma \int_{\Sset} \phivec(\svec') \big(f(\svec ') + g(\svec ')\big)  \de \nonumber \svec'\bigg) \bigg| \nonumber \\
			& = & \bigg| \bm{\varepsilon}_{\pi}^T(\svec) \bigg(\rvec + \gamma \int_{\Sset} \phivec(\svec')  g(\svec' )  \de \nonumber \svec' \bigg)- \bm{\varepsilon}_{\pi}^T(\svec) \bigg(\rvec + \gamma \int_{\Sset} \phivec(\svec') \big(f^*(\svec ') + g(\svec ')\big)  \de \nonumber \svec'\bigg) \bigg| \nonumber \\
			& = & \gamma \bigg| \bm{\varepsilon}_{\pi}^T(\svec)   \int_{\Sset} \phivec(\svec') g(\svec ')  \de \nonumber \svec'\bigg| \nonumber \\
			\implies |g(\svec)| & = & \gamma \bigg| \bm{\varepsilon}_{\pi}^T(\svec)   \int_{\Sset} \phivec(\svec') g(\svec ' )  \de \nonumber \svec'\bigg|. \nonumber
		\end{eqnarray}
		Using Jensen's inequality
		\begin{eqnarray}
			|g(\svec)|& \leq & \gamma \bm{\varepsilon}_{\pi}^T(\svec)   \int_{\Sset} \phivec(\svec')  |g(\svec ') |  \de \nonumber \svec'. \nonumber
		\end{eqnarray}
		Note that since both $f^*$ and $f$ are bounded by $\frac{R_{\text{max}}}{1-\gamma}$ then $|g(\svec)| \leq \frac{2R_{\text{max}}}{1-\gamma}$, thus
		\begin{eqnarray}
			|g(\svec)|& \leq & \gamma \bm{\varepsilon}_{\pi}^T(\svec)   \int_{\Sset} \phivec(\svec')  |g(\svec ') |  \de  \svec' \label{equation:recursion} \\
			& \leq & \gamma  2\frac{R_{\text{max}}}{1-\gamma} \bm{\varepsilon}_{\pi}^T(\svec)   \int_{\Sset} \phivec(\svec')    \de \nonumber \svec' \nonumber \\
			& = & \gamma  2\frac{R_{\text{max}}}{1-\gamma}  \nonumber \\
			\implies |g(\svec)|& \leq & \gamma \frac{2R_{\text{max}}}{1-\gamma} \nonumber \\
			\implies |g(\svec)|& \leq & \gamma^2 \frac{2R_{\text{max}}}{1-\gamma} \quad \quad \text{using \eqref{equation:recursion}}\nonumber \\
			\implies |g(\svec)|& \leq & \gamma^3 \frac{2R_{\text{max}}}{1-\gamma} \quad \quad \text{using \eqref{equation:recursion}}\nonumber \\
			\dots \nonumber \\
			\implies |g(\svec)|& \leq &  0, \nonumber
		\end{eqnarray}
		which is in clear disagreement with the assumption made. Again here a similar procedure shows the same result for the infinite case.
	\end{proof}
\end{proposition}

\paragraph{Proof of Theorem~\ref{theorem:fixedpoint}}
\begin{proof}
	Saying that $\approxx{V}_{\pi}^*$ is a solution for Equation~\eqref{equation:infnpbe} is equivalent to saying
	\begin{equation}
		\approxx{V}_{\pi}^*(\svec) - \bm{\varepsilon}^{\pi}(\svec) \bigg(\rvec + \gamma \int_{\Sset} \phivec(\svec')\approxx{V}_{\pi}^*(\svec')   \de \svec'\bigg) = 0 \quad \quad \forall \svec \in \Sset. \nonumber
	\end{equation}
	We can verify that by simple algebraic manipulation
	\begin{eqnarray}
		& & \approxx{V}_{\pi}^*(\svec) - \bm{\varepsilon}_{\pi}^T(\svec) \bigg(\rvec + \gamma \int_{\Sset} \phivec(\svec')\approxx{V}_{\pi}^*(\svec')   \de \svec'\bigg) \nonumber \\
		& = & \bm{\varepsilon}_{\pi}^T(\svec) \bm{\Lambda}_{\pi}^{-1} \rvec - \bm{\varepsilon}^{\pi}(\svec) \bigg(\rvec + \gamma \int_{\Sset} \phivec(\svec')\bm{\varepsilon}_{\pi}^T(\svec') \bm{\Lambda}_{\pi}^{-1}\rvec   \de \svec'\bigg) \nonumber \\
		& = & \bm{\varepsilon}_{\pi}^T(\svec)\bigg(\bm{\Lambda}_{\pi}^{-1} \rvec - \rvec - \gamma \int_{\Sset} \phivec(\svec')\bm{\varepsilon}_{\pi}^T(\svec') \bm{\Lambda}_{\pi}^{-1}\rvec   \de \svec'\bigg) \nonumber \\
		& = & \bm{\varepsilon}_{\pi}^T(\svec)\Bigg(\bigg(I- \gamma \int_{\Sset} \phivec(\svec')\bm{\varepsilon}_{\pi}^T(\svec')   \de \svec'\bigg)\bm{\Lambda}_{\pi}^{-1}\rvec - \rvec   \Bigg) \nonumber \\
		& = & \bm{\varepsilon}_{\pi}^T(\svec)\Bigg(\bm{\Lambda}_{\pi}\bm{\Lambda}_{\pi}^{-1}\rvec - \rvec   \Bigg) \nonumber \\
		& = & 0.
	\end{eqnarray}
	Since equation~\eqref{equation:infnpbe} has (at least) one solution, Proposition~\ref{proposition:uniqueness} guarantees that the solution ($\approxx{V}_{\pi}^*$) is unique.
\end{proof}

\paragraph{Proof of Theorem~\ref{theorem:ultimate}.}
\begin{proof}
	We perform the derivation for the stochastic policy, however the same derivation applies for the deterministic case almost identically.
	Expanding $\big|\EV_{D}[\overline{V}_D(\svec)] - V^*(\svec)\big|$ using the NPBE and the classic Bellman equation,
	\begin{eqnarray}
		\big|\EV_{D}[\overline{V}_D(\svec)] - V^*(\svec)\big| &= &\Bigg| \EV_D\bigg[\int_{\Sset \times \Aset} \varepsilon_{\pi}(\svec,\zvec, \bvec) \bigg( R_{\zvec, \bvec} + \gamma \int_{\Sset}V_D(\svec')\phi(\svec', \zvec_{\zvec, \bvec}')\de \svec  \bigg) \beta(\zvec, \bvec) \de \zvec \de \bvec \nonumber \bigg] \nonumber \\
		& & - \int_{\Aset} \bigg(\overline{R}(\svec,\avec) + \gamma \int_{\Sset} V^*(\svec')p(\svec'|\svec, \avec)\de \svec' \bigg)\pi(\avec|\svec)\de \avec\Bigg|. \label{equation:expand}
	\end{eqnarray}
	As can be easily verified, $\varepsilon_{\pi}(\svec,\zvec,\bvec)\beta(\zvec,\bvec)$ is a density distribution over $\zvec, \bvec$. Hence Equation~\eqref{equation:expand} can be rewritten
	\begin{eqnarray}
		& & \Bigg|\EV_D\bigg[\int_{\Sset \times \Aset} \varepsilon_{\pi}(\svec,\zvec, \bvec) \bigg( R_{\zvec, \bvec} + \gamma \int_{\Sset}V_D(\svec')\phi(\svec', \zvec_{\zvec, \bvec}')\de \svec'  \bigg) \beta(\zvec, \bvec) \de \zvec \de \bvec \nonumber \bigg] \nonumber \\
		& & - \int_{\Aset} \bigg(\overline{R}(\svec,\avec)  + \gamma \int_{\Sset} V^*(\svec')p(\svec'|\svec, \avec)\de \svec' \bigg)\pi(\avec|\svec)\de \avec\Bigg| \nonumber \\
		& = & \Bigg|\EV_D\bigg[ \int_{\Aset}\frac{\int_{\Sset \times \Aset}\psi(\svec, \zvec)\varphi(\avec, \bvec)\big( R_{\zvec, \bvec}  - \overline{R}(\svec,\avec)\big)\beta(\zvec, \bvec)\de \zvec \de \bvec}{\int_{\Sset, \Aset}\psi(\svec, \zvec)\varphi(\avec, \bvec)\beta(\zvec, \bvec) \de \zvec \de \bvec}  \pi(\avec | \svec) \de \avec \bigg]\nonumber \\
		&  +  & \gamma  \int_{\Aset}\EV_D\bigg[\frac{\int_{\Sset \times \Aset}\psi(\svec, \zvec)\varphi(\avec, \bvec)\big(\int_{\Sset}V_D(\svec')\phi(\svec', \zvec_{\zvec, \bvec}')\de \svec'- \int_{\Sset} V^*(\svec')p(\svec'|\svec, \avec)\de \svec'  \big)\beta(\zvec, \bvec)\de \zvec \de \bvec}{\int_{\Sset, \Aset}\psi(\svec, \zvec)\varphi(\avec, \bvec)\beta(\zvec, \bvec) \de \zvec \de \bvec}\bigg]  \pi(\avec | \svec) \de \avec  \nonumber  \Bigg| \nonumber  \\
		& \leq & \Bigg|\EV_D\bigg[ \int_{\Aset}\underbrace{\frac{\int_{\Sset \times \Aset}\psi(\svec, \zvec)\varphi(\avec, \bvec)\big( R_{\zvec, \bvec}  - \overline{R}(\svec,\avec)\big)\beta(\zvec, \bvec)\de \zvec \de \bvec}{\int_{\Sset, \Aset}\psi(\svec, \zvec)\varphi(\avec, \bvec)\beta(\zvec, \bvec) \de \zvec \de \bvec}}_\text{A}  \pi(\avec | \svec) \de \avec \bigg]\nonumber\Bigg| \\
		&  +  & \gamma  \Bigg|\int_{\Aset}\underbrace{\EV_D\bigg[\frac{\int_{\Sset \times \Aset}\psi(\svec, \zvec)\varphi(\avec, \bvec)\big(\int_{\Sset}V_D(\svec')\phi(\svec', \zvec_{\zvec, \bvec}')\de \svec'- \int_{\Sset} V^*(\svec')p(\svec'|\svec, \avec)\de \svec'  \big)\beta(\zvec, \bvec)\de \zvec \de \bvec}{\int_{\Sset, \Aset}\psi(\svec, \zvec)\varphi(\avec, \bvec)\beta(\zvec, \bvec) \de \zvec \de \bvec}\bigg]}_\text{B}  \pi(\avec | \svec) \de \avec  \nonumber  \Bigg| \nonumber  \\
		& \leq & \text{A}_\text{Bias} + \gamma \text{B}_\text{Bias}. \label{equation:twoterms}
	\end{eqnarray}
	It is evident that the term \textsl{A} is the Nadaraya-Watson kernel regression, as it is possible to observe in the beginnin of the proof at page twelve of \cite{tosatto_upper_2020}, therefore Theorem~\ref{theorem:biasnadaraya} applies
	\begin{eqnarray}
		\text{A}_\text{Bias} & = & \quad \frac{L_R \sum_{k=1}^d \hvec_k \Bigg(\prod_{i\neq k}^d \e{\frac{L_{\beta}^2 \hvec_i^2}{2}}\Bigg(1 +  \erf\bigg(\frac{\hvec_i L_{\beta}}{\sqrt{2}}\bigg) \Bigg)\Bigg)  \Bigg( \frac{1}{\sqrt{2 \pi} } + L_{\beta}\hvec_k \frac{\e{\frac{L_{\beta}^2 \hvec_k^2}{2}}}{2}\Bigg(1 + \erf\bigg(\frac{\hvec_k L_{\beta}}{\sqrt{2}}\bigg) \Bigg)\Bigg)}{\prod_{i=1}^d  \e{\frac{L_{\beta}^2 h_i^2}{2}}\Bigg(1 - \erf\bigg(\frac{\hvec_i L_{\beta}}{\sqrt{2}}\bigg) \Bigg)}\nonumber,  \label{bias}
	\end{eqnarray}
	where $\hvec = [\hvec_{\psi},\hvec_{\varphi}]$ and $d = d_s + d_a$.	\\
	Returning to the estimate of $\text{B}_\text{Bias}$
	\begin{eqnarray}
		& &  \Bigg|\int_{\Aset}\EV_D\bigg[\frac{\int_{\Sset \times \Aset}\psi(\svec, \zvec)\varphi(\avec, \bvec)\big(\int_{\Sset}V_D(\svec')\phi(\svec', \zvec_{\zvec, \bvec}')\de \svec'- \int_{\Sset} V^*(\svec')p(\svec'|\svec, \avec)\de \svec'  \big)\beta(\zvec, \bvec)\de \zvec \de \bvec}{\int_{\Sset, \Aset}\psi(\svec, \zvec)\varphi(\avec, \bvec)\beta(\zvec, \bvec) \de \zvec \de \bvec}\bigg] \pi(\avec | \svec) \de \avec  \nonumber  \Bigg| \nonumber \\
		&= &  \Bigg|\int_{\Aset}\frac{\int_{\Sset \times \Aset}\psi(\svec, \zvec)\varphi(\avec, \bvec)\big(\int_{\Sset}\EV\big[V_D(\svec')\phi(\svec', \zvec_{\zvec, \bvec}') \big] \de\svec'- \int_{\Sset} V^*(\svec')p(\svec'|\svec, \avec)\de \svec'  \big)\beta(\zvec, \bvec)\de \zvec \de \bvec}{\int_{\Sset, \Aset}\psi(\svec, \zvec)\varphi(\avec, \bvec)\beta(\zvec, \bvec) \de \zvec \de \bvec} \pi(\avec | \svec) \de \avec  \nonumber  \Bigg| \nonumber
	\end{eqnarray}

	One my ask whether the terms in  $\EV[V_D(\svec')\phi(\svec', \zvec_{\zvec, \bvec}')]$ are uncorrelated. The answer it is affirmative, since, even if $V_D$ depends by $\zvec_{\zvec, \bvec}$ (integral in Equation~\eqref{equation:infnpbe}), this corresponds only in the variation of a single point in the integral, and therefore the overall estimate does not change. This argument, however, does not immediately hold for the case of an infinitesimal bandwidth, and therefore we provide the results for that case separately.
	\paragraph{For Finite Bandwidth:}
	\begin{eqnarray}
		& &  \Bigg|\int_{\Aset}\frac{\int_{\Sset \times \Aset}\psi(\svec, \zvec)\varphi(\avec, \bvec)\big(\int_{\Sset}\EV\big[V_D(\svec')\phi(\svec', \zvec_{\zvec, \bvec}')\big]\de \svec'- \int_{\Sset} V^*(\svec')p(\svec'|\svec, \avec)\de \svec'  \big)\beta(\zvec, \bvec)\de \zvec \de \bvec}{\int_{\Sset, \Aset}\psi(\svec, \zvec)\varphi(\avec, \bvec)\beta(\zvec, \bvec) \de \zvec \de \bvec} \pi(\avec | \svec) \de \avec  \nonumber  \Bigg| \nonumber\\
		& \leq & \max_{\svec, \avec}\Bigg|\frac{\int_{\Sset \times \Aset}\psi(\svec, \zvec)\varphi(\avec, \bvec)\big(\int_{\Sset\times \Sset}\overline{V}(\zvec')\phi(\zvec', \svec')p(\svec'|\svec,\avec)\de \svec'\de \zvec'- \int_{\Sset} V^*(\svec')p(\svec'|\svec, \avec)\de \svec'  \big)\beta(\zvec, \bvec)\de \zvec \de \bvec}{\int_{\Sset, \Aset}\psi(\svec, \zvec)\varphi(\avec, \bvec)\beta(\zvec, \bvec) \de \zvec \de \bvec}\Bigg| \nonumber \\
		& = & \max_{\svec, \avec}\Bigg|\frac{\int_{\Sset \times \Aset}\psi(\svec, \zvec)\varphi(\avec, \bvec)\big(\int_{\Sset}\int_{\Sset}\big(\overline{V}(\zvec')\phi(\zvec', \svec')-V^*(\svec')\big)p(\svec'|\svec,\avec)\de \svec'\de \zvec'  \big)\beta(\zvec, \bvec)\de \zvec \de \bvec}{\int_{\Sset, \Aset}\psi(\svec, \zvec)\varphi(\avec, \bvec)\beta(\zvec, \bvec) \de \zvec \de \bvec}\Bigg| \nonumber \\
		& \leq & \max_{\svec, \avec, \svec'}\Bigg|\frac{\int_{\Sset \times \Aset}\psi(\svec, \zvec)\varphi(\avec, \bvec)\big(\int_{\Sset}\overline{V}(\zvec')\phi(\zvec', \svec')-V^*(\svec')\de \zvec'  \big)\beta(\zvec, \bvec)\de \zvec \de \bvec}{\int_{\Sset, \Aset}\psi(\svec, \zvec)\varphi(\avec, \bvec)\beta(\zvec, \bvec) \de \zvec \de \bvec}\Bigg| \nonumber \\
		& = & \max_{\svec, \avec, \svec'}\Bigg|\frac{\int_{\Sset \times \Aset}\psi(\svec, \zvec)\varphi(\avec, \bvec)\beta(\zvec, \bvec)\de \zvec \de \bvec}{\int_{\Sset, \Aset}\psi(\svec, \zvec)\varphi(\avec, \bvec)\beta(\zvec, \bvec) \de \zvec \de \bvec}\bigg(\int_{\Sset}\overline{V}(\zvec')\phi(\zvec', \svec')-V^*(\svec')\de \zvec'  \bigg) \Bigg|\nonumber \\
		& = & \max_{\svec, \avec, \svec'}\bigg|\int_{\Sset}\overline{V}(\zvec')\phi(\zvec', \svec')-V^*(\svec')\de \zvec'  \bigg|\nonumber \\
		& = & \max_{\svec, \avec, \svec'}\bigg|\int_{\Sset}\overline{V}(\svec'+\lvec)\phi(\svec+\lvec, \svec')-V^*(\svec')\de \lvec  \bigg|. \label{equation:finitesamples}
	\end{eqnarray}
	Note that
	\begin{equation}
		\phi(\svec' + \lvec, \svec') = \prod_{i=1}^{d_s}\frac{e^{- \frac{l_i^2}{2h^2_{\phi,i}}}}{\sqrt{2\pi h^2_{\phi,i}}}, \nonumber
	\end{equation}
	thus
	\begin{eqnarray}
		&  &  \max_{\svec, \avec, \svec'}\bigg|\int_{\Sset}\overline{V}(\svec'+\lvec)\phi(\svec+\lvec, \svec')-V^*(\svec')\de \lvec  \bigg|\nonumber\\
		& \leq & \max_{\svec, \avec, \svec'}\bigg| \overline{V}(\svec')-V^*(\svec')\bigg| + \int_{\Sset} L_{V}\bigg(\sum_{i=1}^{d_s}|l_i|\bigg)\prod_{i=1}^{d_s}\frac{e^{- \frac{l_i^2}{2h^2_{\phi,i}}}}{\sqrt{2\pi h^2_{\phi,i}}}\de. \lvec \nonumber
	\end{eqnarray}
	Using Proposition~\ref{prodsumint}
	\begin{eqnarray}
		&  & \max_{\svec, \avec, \svec'}\bigg| \overline{V}(\svec')-V^*(\svec')\bigg| + L_{V} \int_{\Sset} \bigg(\sum_{i=1}^{d_s}|l_i|\bigg)\prod_{i=1}^{d_s}\frac{e^{- \frac{l_i^2}{2h^2_{\phi,i}}}}{\sqrt{2\pi h^2_{\phi,i}}}\de \lvec \nonumber \\
		& =  & \max_{\svec, \avec, \svec'}\bigg| \overline{V}(\svec')-V^*(\svec')\bigg| +L_{V} \sum_{k=1}^{d_s}\bigg(\prod_{i\neq k}^{d_s}\int_{-\infty}^{+\infty} \frac{e^{- \frac{l_i^2}{2h^2_{\phi,i}}}}{\sqrt{2\pi h^2_{\phi,i}}}\de l_i\bigg)\int_{-\infty}^{+\infty}|l_k| \frac{e^{- \frac{l_k^2}{2h^2_{\phi,k}}}}{\sqrt{2\pi h^2_{\phi,k}}} \de l_k \nonumber \\
		& =  & \max_{\svec, \avec, \svec'}\bigg| \overline{V}(\svec')-V^*(\svec')\bigg| +L_{V}2 \sum_{k=1}^{d_s}\int_{0}^{+\infty}l_k \frac{e^{- \frac{l_k^2}{2h^2_{\phi,k}}}}{\sqrt{2\pi h^2_{\phi,k}}} \de l_k \nonumber \\
		& =  & \max_{\svec, \avec, \svec'}\bigg| \overline{V}(\svec')-V^*(\svec')\bigg| +L_{V} \sum_{k=1}^{d_s}\frac{h_{\phi,k}}{\sqrt{2 \pi}} \nonumber \\
	\end{eqnarray}
	which means that when $\hvec$ not infinitesimal
	\begin{eqnarray}
		& & \bigg| \overline{V}(\svec)-V^*(\svec)\bigg| \leq \text{A}_\text{Bias} + \gamma \bigg(\max_{\svec, \avec, \svec'}\bigg| \overline{V}(\svec')-V^*(\svec')\bigg| +L_{V} \sum_{k=1}^{d_s}\frac{h_{\phi,k}}{\sqrt{2 \pi}}\bigg).  \nonumber
	\end{eqnarray}
	It is however known that $\big|\overline{V}(\svec)-V^*(\svec)\big| \leq 2\frac{R_{\text{max}}}{1-\gamma}$, thus
	\begin{eqnarray}
		& & \bigg| \overline{V}(\svec)-V^*(\svec)\bigg| \leq \text{A}_\text{Bias} + \gamma \bigg(\max_{\svec, \avec, \svec'}\bigg| \overline{V}(\svec')-V^*(\svec')\bigg| +L_{V} \sum_{k=1}^{d_s}\frac{h_{\phi,k}}{\sqrt{2 \pi}}\bigg)  \label{equation:recursion1}  \\
		& & \bigg| \overline{V}(\svec)-V^*(\svec)\bigg| \leq \text{A}_\text{Bias} + \gamma \bigg(2\frac{R_{\text{max}}}{1-\gamma} +L_{V} \sum_{k=1}^{d_s}\frac{h_{\phi,k}}{\sqrt{2 \pi}}\bigg) \nonumber \\
		\implies & &  \bigg| \overline{V}(\svec)-V^*(\svec)\bigg| \leq \text{A}_\text{Bias} + \gamma \bigg(\text{A}_\text{Bias} + \gamma \bigg(2\frac{R_{\text{max}}}{1-\gamma} +L_{V} \sum_{k=1}^{d_s}\frac{h_{\phi,k}}{\sqrt{2 \pi}}\bigg) +L_{V} \sum_{k=1}^{d_s}\frac{h_{\phi,k}}{\sqrt{2 \pi}}\bigg)  \qquad \text{using Equation~\eqref{equation:recursion1}} \nonumber \\
		\implies & &  \bigg| \overline{V}(\svec)-V^*(\svec)\bigg| \leq \sum_{t=0}^{\infty}\gamma^t \bigg(\text{A}_\text{Bias} + \gamma L_{V} \sum_{k=1}^{d_s}\frac{h_{\phi,k}}{\sqrt{2 \pi}} \bigg)  \qquad \text{using Equation~\eqref{equation:recursion1}} \nonumber \\
		\implies & &  \bigg| \overline{V}(\svec)-V^*(\svec)\bigg| \leq  \frac{1}{1-\gamma} \bigg(\text{A}_\text{Bias} + \gamma L_{V} \sum_{k=1}^{d_s}\frac{h_{\phi,k}}{\sqrt{2 \pi}} \bigg). \nonumber 
	\end{eqnarray}
	\paragraph{For Infinitesimal Bandwidth:}
	In the case of an infinitesimal bandwidth note that, even if $V_D$ and $\phi$ are correlated the overall integral reduces only on a single point, and the same argument made in the case of finite bandwidth applies,
	\begin{eqnarray}
		\int_{\Sset}\EV\big[V_D(\svec')\phi(\svec', \zvec_{\zvec, \bvec}')\big]\de  \svec' = \EV\bigg[\int_{\Sset}V_D(\svec')\phi(\svec', \zvec_{\zvec, \bvec}'\de  \svec') \de \svec' \bigg] = \EV\big[V_D( \zvec_{\zvec, \bvec}')\big]
		=  \int_{\Sset} \overline{V}_D(\svec')p(\svec'|\svec,\avec)\de \svec'. \nonumber
	\end{eqnarray}
	It follows that, proceeding similarly to Equation~\eqref{equation:finitesamples}, we obtain
	\begin{eqnarray}
		\big|\EV_{D}[\overline{V}_D(\svec)] - V^*(\svec)\big| \leq \max_{\svec, \avec, \svec'}\bigg|\overline{V}(\svec')-V^*(\svec') \bigg|,
	\end{eqnarray}
	which yields
	\begin{equation}
		\bigg| \overline{V}(\svec)-V^*(\svec)\bigg| \leq  \frac{1}{1-\gamma} \text{A}_\text{Bias}.
	\end{equation} 
\end{proof}

\section{Empirical Evaluation Detail}

\subsection{Linear Quadratic Regulator Experiment}\label{appendix:gradient_lqr}

Here we detail the experiment presented in Figure~\ref{figure:gradient}. We use a discrete infinite-horizon discounted Linear Quadratic Regulator system of the form
\begin{align}
\max_{\vec{x}_t, \vec{u}_t} \, & J = \, \frac{1}{2} \sum_{t=0}^{\infty} \gamma^t \left( \vec{x}_t^{\top} \mathbf{Q} \vec{x}_t + \vec{u}_t^{\top} \mathbf{R} \vec{u}_t \right) \nonumber \\
%\st
& \vec{x}_{t+1}  =  \Avec \vec{x}_t + \mathbf{B} \vec{u}_t \quad \forall t, \nonumber 
\end{align}
where $\vec{x}_t \in \mathbb{R}^{d_{x}}$, $\vec{u}_t \in \mathbb{R}^{d_u}$, $\mathbf{Q} \in \mathbb{R}^{d_x \times d_x}$, $\mathbf{R} \in \mathbb{R}^{d_u \times d_u}$, $\Avec \in \mathbb{R}^{d_x \times d_x}$, $\mathbf{B} \in \mathbb{R}^{d_x \times d_u}$, $\gamma \in [0, 1)$ and $\vec{x}_0$ given. 

In this example we use consider a 2-dimensional problem with the following quantities
\begin{align*}
\Avec & =\left[\begin{array}{cc}
1.2 & 0\\
0 & 1.1
\end{array}\right] \quad \quad \quad  \mathbf{B}=\left[\begin{array}{cc}
0.1 & 0\\
0 & 0.2
\end{array}\right]\\
\mathbf{Q} & =\left[\begin{array}{cc}
-0.5 & 0\\
0 & -0.25
\end{array}\right] \quad \mathbf{R}=\left[\begin{array}{cc}
0.01 & 0\\
0 & 0.01
\end{array}\right]\\
\vec{x}_0 & = \left[ \begin{array}{c}
1 \\
1
\end{array} \right]
\quad \quad 
\gamma  = 0.9.
\end{align*}

For this LQR problem we impose a linear controller as a diagonal matrix
\begin{align}
\mathbf{K} = \left[ \begin{array}{cc}
k_1 & 0  \\
0 & k_2
\end{array} \right]. \label{eq:lqr_diagonal_policy}
\end{align}

\subsubsection{Deterministic Experiment}

For each dataset we run 100 trajectories of 30 steps. Each trajectory is generated by following the dynamics of the described LQR and using at each time step a fixed policy initialized as
\begin{align}
\mathbf{K} = \left[ \begin{array}{cc}
k_1 + \varepsilon & \varepsilon  \\
\varepsilon & k_2 + \varepsilon 
\end{array} \right], \; \varepsilon \sim \mathcal{N}(0, 1), \nonumber
\end{align}
where $k_1 = 0.7$ and $k_2 = -0.7$.

NOPG-D optimized for each dataset a policy encoded as in \eqref{eq:lqr_diagonal_policy} with: learning rate $0.5$ with ADAM optimizer; bandwidths (on average) for the state space  $\vec{h}_{\psi} = [0.03, 0.05]$ and for the action space $\vec{h}_{\varphi} = [0.33, 0.27]$; discount factor $\gamma=0.9$; and keeping 5 elements per row after sparsification of the $\mathbf{P}$ matrix.

DPG optimized for each dataset a policy encoded as in \eqref{eq:lqr_diagonal_policy} with: learning rate $0.5$ with ADAM optimizer; $Q$-function encoded as $Q(\vec{x}, \vec{u}) = \vec{x}^{\top} \mathbf{Q} \vec{x} + \vec{u}^{\top} \mathbf{R} \vec{u}$ (with $\mathbf{Q}$ and $\mathbf{R}$ to be learned); discount factor $\gamma=0.9$; two target networks are kept to stabilize learning and soft-updated using $\tau = 0.01$ (similar to DDPG).


\subsubsection{Stochastic Experiment} 

For each dataset we run 100 trajectories of 30 steps. Each trajectory is generated by following the dynamics of the described LQR, and using at each time step a stochastic policy as
\begin{align}
\vec{u}_t = \mathbf{K}  \vec{x}_t + \vec{\varepsilon}, \; \vec{\varepsilon} \sim \mathcal{N} \left( \vec{\mu} = \vec{0}, \mathbf{\Sigma} = \textrm{diag}( 0.01, 0.01) \right), \label{eq:lqr_diagonal_policy_stochastic}
\end{align}
where $\mathbf{K} = \textrm{diag}(0.35, -0.35)$.

NOPG-S optimized for each dataset a policy encoded as in \eqref{eq:lqr_diagonal_policy_stochastic} with: learning rate $0.25$ with ADAM optimizer; bandwidths (on average) for the state space $\vec{h}_{\psi} = [0.008, 0.003]$ and for the action space $\vec{h}_{\varphi} = [0.02, 0.02]$; discount factor $\gamma=0.9$; and keeping 10 elements per row after sparsification of the $\mathbf{P}$ matrix.

PWIS optimized for each dataset a policy encoded as in \eqref{eq:lqr_diagonal_policy_stochastic} with: learning rate $2.5 \times 10^{-4}$ with ADAM optimizer; and discount factor $\gamma=0.9$. 



\subsection{Other Experiments Configurations}\label{appendix:experiments_configs}

We use a policy encoded as neural network with parameters $\vec{\theta}$. A deterministic policy is encoded with a neural network $\action = f_{\vec{\theta}}(\state)$. The stochastic policy is encoded as a Gaussian distribution with parameters determined by a neural network with two outputs, the mean and covariance. In this case we represent by $f_{\vec{\theta}}(\state)$ the slice of the output corresponding to the mean and by $g_{\vec{\theta}}(\state)$ the part of the output corresponding to the covariance. 
%In some algorithms we use a latent representation as part of the policy and value function networks, denoted by $\vec{z} = h_{\vec{\theta}}(\state)$, which is then linearly transformed to give the Gaussian policy parameters or to compute the value function.

NOPG can be described with the following hyper-parameters

\begin{longtable}{l l}
	\textbf{NOPG Parameters} & Meaning\\
	\hline
	dataset sizes & number of samples contained in the dataset used for training \\        
	discount factor $\gamma$ & usual discount factor in infinite horizon MDP \\
	state $\vec{h}_{\textrm{factor}}$ & constant used to decide the bandwidths for the state-space \\
	action $ \vec{h}_{\textrm{factor}}$ & constant used to decide the bandwidths for the action-space \\
	policy & parametrization of the policy\\
	policy output & how is the output of the policy encoded \\               
	learning rate  & the learning rate and the gradient ascent algorithm used \\
	$N_{\pi}^{\textrm{MC}}$ (NOPG-S) & number of samples drawn to compute the integral $\bm{\varepsilon}_{\pi}(\state)$ with MonteCarlo sampling \\
	$N_{\phi}^{\textrm{MC}}$ & number of samples drawn to compute the integral over the next state $\int \phi(\state')\de \state'$\\
	$N_{\mu_0}^{\textrm{MC}}$ & number of samples drawn to compute the integral over the initial \\
	&  distribution $\int \hat{V}_{\pi}(\state) \mu_{0}(\state) \de \state$ \\
	policy updates & number of policy updates before returning the optimized policy \\
	\hline
\end{longtable}

A  few considerations about NOPG parameters. If $N_{\phi}^{\textrm{MC}}=1$ we use the mean of the kernel $\phi$ as a sample to approximate the integral over the next state. When optimizing a stochastic policy represented by a Gaussian distribution, we set and linearly decay the variance over the policy optimization procedure. The kernel bandwidths are computed in two steps: first we find the best bandwidth for each dimension of the state and action spaces using cross validation; second we multiply each bandwidth by an empirical constant factor ($\vec{h}_{\textrm{factor}}$). This second step is important to guarantee that the state and action spaces do not have a zero density. For instance, in a continuous action environment, when sampling actions from a uniform grid we have to guarantee that the space between the grid points have some density. The problem of estimating the bandwidth in kernel density estimation is well studied, but needs to be adapted to the problem at hand, specially with a low number of samples. We found this approach to work well for our experiments but it still can be improved.


\subsubsection{Pendulum with Uniform Dataset}
\input{experiments/Pendulum_uniform_dataset_configs.tex}

\input{experiments/Pendulum_uniform_configs.tex}

\subsubsection{Pendulum with Random Agent}
\input{experiments/Pendulum_random_configs.tex}

\subsubsection{Cart-pole with Random Agent}
\input{experiments/Cartpole_random_configs.tex}

\subsubsection{Mountain Car with Human Demonstrator}
\input{experiments/MountainCar_random_configs.tex}


%\end{adjustwidth}
